# Supplementary material for: Proton-Boron Fusion Yield Increased by Orders of Magnitude with Foam Targets
Source: arXiv:2308.10878 source file (2023-08-21)
Supplement: Supplementary file 1 [file SM_proton_boron_fusion.pdf]

# Supplemental materials

## I. FOAM TARGET FABRICATION AND PLASMA CHARACTERIZATION OF TEMPERATURE AND DENSITY

The foam target doped 20% natural boron is fabricated with in-situ consolidation technology by the staff of Laser Fusion Research Center. Firstly, micron-scale boron particles are physically doped into a low-density (~ 2mg/cm$^3$) cellulose triacetate solution (TAC, $C_9H_{16}O_8$). Secondly, with the boron powders fully dispersed, the solution is rapidly cooled to a gel state under the low-temperature condition (~ −6°C). In this sol-gel stage, prompt cooling and gelatinization can inhibit the boron particles to settle and agglomerate. Finally, via the supercritical drying technique, the CHO foam with boron homogeneously doped is obtained. Through measuring the mass and size of reference samples with regular 3D sponge shape, the density and the boron content are determined to be 2.0±0.1 mg/cm$^3$ and (20 ± 1)%, respectively. The density is validated through analysing the stopping power of the 1 mm foam interacting with 5.16 MeV, 5.49 MeV, and 5.80 MeV $\alpha$ particles from $^{239}$Pu, $^{241}$Am and $^{244}$Cm, respectively. Via comparing the measured energy losses of the $\alpha$ particles with the SRIM predictions, the foam density is determined as 1.9±0.3 mg/cm$^3$.

The temperatures of the gold hohlraum and CHO-B plasma are characterized by measuring their radiation spectra [30]. A transmission grating spectrometer (TGS) is coupled to a calibrated image plate (IP, type BAS-TR) for hohlraum radiation measurement. Note that the TGS is outfitted with a single-order diffraction grating (1000 lines/mm) and a slit of 100 $\mu$m to filter high-order components with moderate diffraction efficiency both in the visible light and soft X-ray regions, as well as the extreme ultraviolet regions [S1]. The raw data of the TGS is shown in Fig. 1(a). The central part is the zero order of the diffraction. The first-order diffraction is analysed to reconstruct the emission spectrum, which is pressented in Fig. 1(b). The spectral resolution is $\delta\lambda$ = 0.16 nm at 12.5 nm. The emission spectrum can be well approximated by Planckian distribution with maximum intensity at $\lambda_{max}$ = 13.3 nm, corresponding to a black-body radiation temperature of 19 eV.

To ensure the plasma is fully heated during the proton-boron fusion reaction, temporal evolution of the soft X-ray flux (<400 eV) generated by the hohlraum is measured using an X-ray diode (XRD) with carbon cathodes covered by a Al filter. The duration of the hohlraum soft X-ray radiation is about 6 ns, during which the foam is continually heated. A pinhole camera (PH) is used to characterize the gold hohlraum plasma and the resulting plasma [30]. Hence, the proton beam is synchronized to arrive at the target with 8 ns delay after triggering the heating process in the experimental measurement. The temperature of the CHO-B plasma is diagnosed by recording the emission spectra via using a high-resolution flat-field grating spectrometer with 1200 lines/mm. Spectrum dominated by oxygen lines in the range of 12-23 nm recorded with IP is shown in Fig. 2. The wavelength accuracy is about 0.003 nm and the energy resolution is $\delta\lambda$ = 0.06 nm at 15 nm with a collimation-slit width of 0.2 mm. When the plasma is in the local thermodynamic equilibration, the intensities of emission lines meet $\ln \frac{I_{mm}\lambda_{mn}}{A_{mn}g_m} = -\frac{E_m}{kT_e} + C$, where $I_{mm}$ and $\lambda_{mn}$ are the photon intensity and wavelength emitted when the electron transits from upper shell $m$ to lower shell $n$, C is a constant, $E_m$, $T_e$, $k$, $A_{mn}$ and $g_m$ are the electron binding energy in upper level, electron temperature, Boltzmann constant, transitional probability and statistic weight, respectively [S2]. Via performing linear fitting of $\ln \frac{I_{mm}\lambda_{mn}}{A_{mn}g_m}$ vs. $E_m$ for oxygen lines, the electron temperature is determined to be around 17 eV.

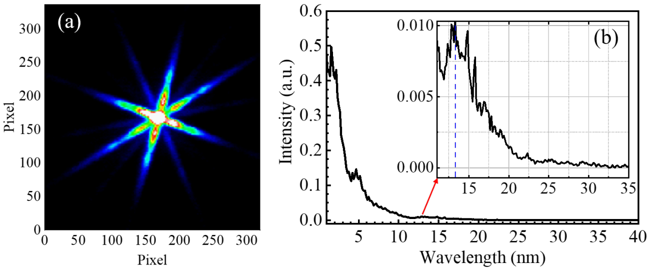


FIG. 1. (a) The raw image recorded by the IP of TGS. (b) The measured radiation spectrum of gold hohlraum.

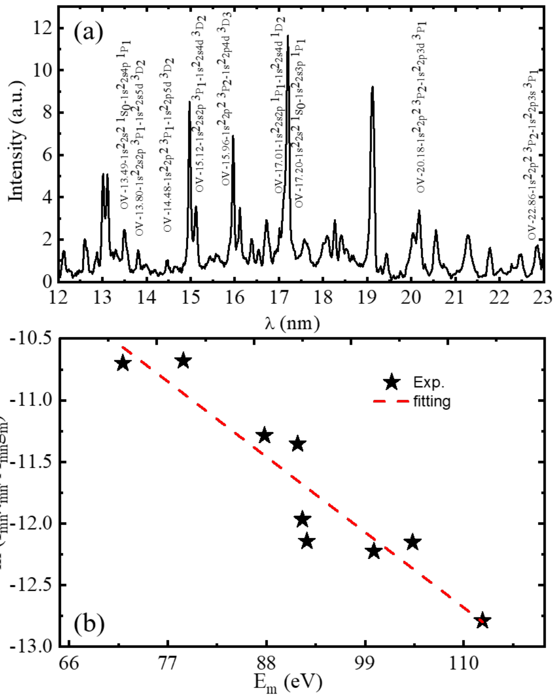


FIG. 2. (a) Emission lines of CHO-B plasma in range of 12-23 nm, dominated by oxygen lines. (b) Saha-Boltzmann plotting of the emission lines. The experimental data (symbols) are linearly fitted (dashed line).

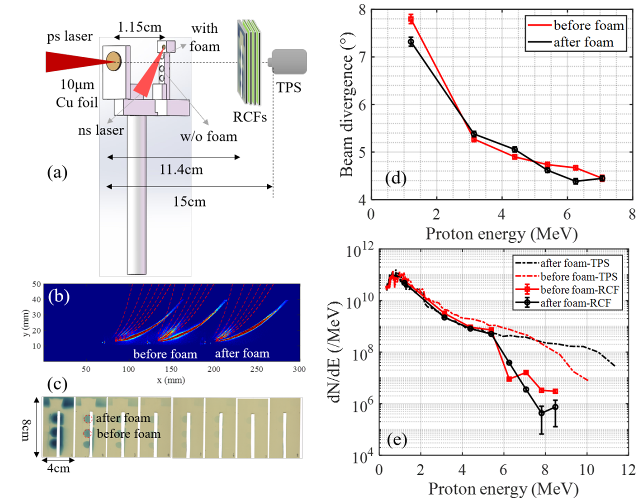


FIG. 3. (a) Experimental setup for the measurement of incident and passed through proton beams with respect to foam targets. (b) and (c) The scanned raw energy spectra and spatial-intensity distributions of the proton beam measured by the multi-channel TPS and the RCF stack, respectively. The middle curve or distribution indicates the protons passing through the empty hole, i.e., the incident protons (before the target), while the right curve or the top distribution denotes the protons passing through the foam target (after the target). (d) The proton beam divergence vs. its energies before (red curve) and after (black curve) passing through the target. The error bars correspond to uncertainties in beam radius fitting. (e) The corresponding proton energy spectra from the TPS (dashed) and RCF stack (solid), respectively. The error bars show the level of uncertainty in the calibration of the RCF stack.

As investigated previously, the foam target approximately keeps its initial mass density for more than 10 ns after heating. Under such an assumption, the ion charge state distributions are calculated by using the collisional-radiative code FLYCHK. The average ionization degree of CHO-B foam is around $C_9^{3.8+}H_{16}^{0.98+}O_8^{4.5+}B_{5.8}^{2.9+}$ at the electron temperature of 16.8±1.1eV, and the corresponding free electron density is $4.0 \pm 0.3 \times 10^{20}$cm$^{-3}$. This gives the $^{11}$B density of $\sim 1.8 \times 10^{19}$cm$^{-3}$. Here the relative error is 7%.

## II. MEASUREMENTS OF THE INCIDENT PROTON BEAM PROPERTIES

One of the key factors for the proton-boron fusion reaction is the measurement of incident proton beam properties, mainly the proton energy $E_p$ and number $N_p$. In the experiment, as shown in Fig. 3 (a), the spatial-intensity distributions and energy spectra of the proton beams are meaured by a calibrated RCF stack (type HD-V2) and a multi-channel Thomson parabola spectrometer (TPS) in conjunction with IP detector with the energy range of $E_p \geq 1.2$ MeV and $0.3 \leq E_p \leq 8$ MeV, respectively. In order to obtain the proton beam energy spectra before and after passing through the target in one laser shot, we design a target holder with two symmetrically distributed holes in relative to beam incidence. The diameter of the holes is 1 mm. One of the upper hole is filled with the foam and the other middle hole is empty to allow the protons, which serves as reference incident protons, passing through without any disturbance simultaneously. The distance of the two holes is 2 mm with a half angle of 5° along the copper target normal direction. Since the intensity distribution of the proton beam generated by laser-driven TNSA at small solid angle range is nearly homogenous, the incident protons into the foam target can be measured via through the middle empty hole [see Figs. 3 (b) and (c)].

Via calculating the total dose in each radiochromic film, the energy spectra of the proton beam before and after the foam target can be extracted, which are shown in solid curves in Fig. 3 (e). Meanwhile, the beam energy spectra can also be obtained by the TPS with an acceptance angle of $1.4 \times 10^{-6}$ sr. Considering the whole beam size or solid angle, the beam divergence angles as a function of its energies are also calculated via beam radius fitting with eleven points recorded on the RCF stack [see Fig. 3 (c) and (d)]. Hence, the energy spectra of the incident and passed through proton beams by TPS can be acquired, which similarly corresponds to those from the RCF stack [see Fig. 3 (e)]. Note that the beam number at high energy range of $E_p \geq 5.4$ MeV from the TPS are higher than those from the RCF stack. This is because the former is mainly measured from the beam central region with higher intensity. Thus, the total proton number is counted by combining the TPS ($0.3 \leq E_p \leq 1.2$ MeV) and RCF stack ($E_p \geq 1.2$ MeV) results. The combined energy spectra and total numbers $N_p$ of the incident proton beams for the exampled three cases are shown in Fig. 2 (a) and listed in Table I in the paper, respectively. Considering uncertainties in RCF calibration, beam radius fitting and uniform of whole beam spatial intensity in the TPS measurement, the error bars of the incident proton number are no more than ±13%.

## III. CALIBRATION OF CR39 TRACK DETECTORS FOR $\alpha$ PARTICLES

To calibrate the response of CR39 track detectors to $\alpha$ particles, we used a collimated standard $^{241}$Am radioactive source which mainly emits 5.49 MeV $\alpha$ particles. The CR39 track detector was filtered with Al foils of different thicknesses from 5 to 20 $\mu$m in order to realize a a calibration at different energies. For our calibration, we selected $\alpha$ particles from 1.38 MeV to 5.49 MeV. The evolution of the $\alpha$-particle track diameters as a function of its energy is shown in Fig. 4, after 3 h etching in a 6 mol/L NaOH solution with a constant temperature of 80°C. We see that the track diameter of the $\alpha$ particles within achieved energies was between 9 and 12 $\mu$m.

## IV. MEAUREMENTS OF $\alpha-$ PARTICLE YIELDS VIA USING THE CR39 DETECTORS COVERED BY AL FOILS

Figures 5 (a) and (b) show an example of raw particle tracks recorded on the CR39 detectors covered by Al foils of thickness from 5 $\mu$m to 40 $\mu$m after 3 h etching for the plasma target case

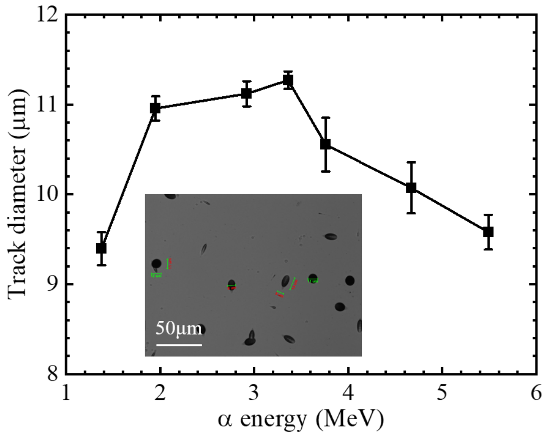


FIG. 4. Calibration curve of CR39 detectors for $\alpha$-particles with track diameters as a function of its energy after 3 h of etching. The error bars are determined from the statistical uncertainties in the measured track diameters. The inset shows the raw sample image of $\alpha$-particle tracks on the CR39 detector without Al foil.

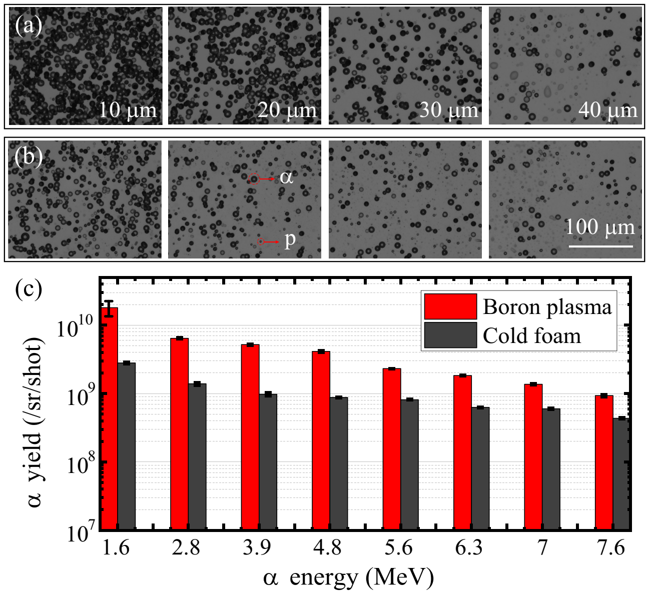


FIG. 5. Typical images of $\alpha$ particle tracks on CR39 detectors positioned at 52°, covered with 10 $\mu$m, 20 $\mu$m, 30 $\mu$m and 40 $\mu$m-thick Al foils after 3 h of etching from (a) boron plasma and (b) cold foam targets, respectively. (c) The corresponding histograms of the $\alpha$-particle energy spectra for statistical regions satisfying $E > E_{cut}$. Here, $E_{cut}$ represents the cut-off energy of $\alpha$ particles through one thickness of Al foil, i.e., the stopping range. The error bars show the statistical uncertainties in $\alpha$-particle yield. The transparent pink column bars denote the raw particle tracks on CR39 detectors to be saturated with larger errors. The CR39 detectors are covered by Al foils of different thickness in $5-40$ $\mu$m.

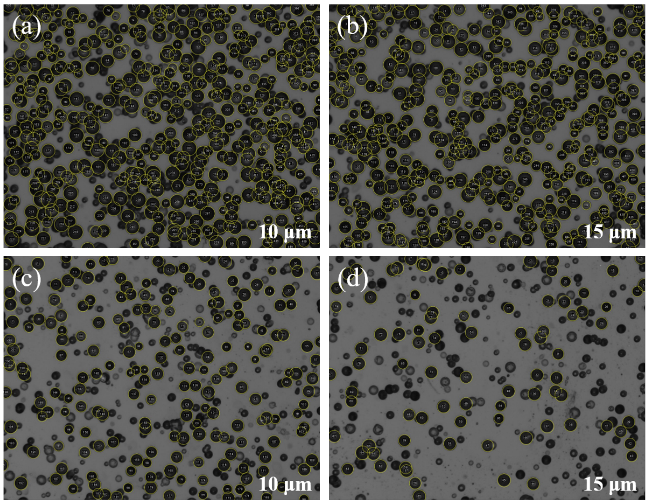


FIG. 6. Several labeled images of particle tracks on CR39 detectors covered with 10 $\mu$m and 15 $\mu$m from (a)-(b) boron plasma and (c)-(d) cold foam targets, respectively.

and non-heated foam target case, respectively. The detectors were placed at a scattering angle of 52°. The thinnest (5 $\mu$m) Al foil predominantly filters low-energy $\alpha$ particles and other ions to reduce the flux density on the CR39 detector. Protons above 750 keV and $\alpha$ particles with energy above 2.8 MeV are transmitted in the case of a 10 $\mu$m-thick Al foil. In this case, the signal is significantly high with partially overlapping tracks. With thicker Al foils, the recorded particle tracks on the detector can be clearly distinguished. Heavy ions, such as carbon and copper, generated via the TNSA mechanism, were almost completely filtered by the 15 $\mu$m-thick Al foil. Comparing the cases of plasma and cold foam targets, the flux in the plasma case is always higher. This clearly indicates that the $\alpha$-particle yield is enhanced in the plasma situation. Via counting the particles with the energy above the corresponding filter cutoff ($E > E_{cut}$), the obtained $\alpha$-particle yield from the plasma are all higher than those in the case of cold foam. Note that the raw particle tracks recorded on the CR39 detectors for thinner filter cases are partially overlapped. To ensure the accuracy of the data, we meaure and label all the relevant particles on several raw fields of view by using the software ImageJ, as shown in Fig. 6 [(a)-(b) for plasma cases and (c)-(d) for foam cases]. Then the $\alpha$ particles can be counted based on the track diameter, circularity and gray level.

## V. CALCULATIONS AND SIMULATIONS OF THE PROTON-BORON FUSION REACTION BASED ON THE BEAM-TARGET SCHEME

Generally, the $\alpha$-particle yield per steradian based on the beam-target reaction can be calculated by the relation $N_\alpha = 3N_pP/4\pi$, where $P(E) = n_B\int_{E_{in}}^{E_{out}}\sigma(E)(\frac{dE}{dx})^{-1}dE = n_B\int_0^{\Delta x}\sigma[E(x)]dx$ is the reaction fusion probability at proton energy $E$. Here, $n_B \simeq 1.8\times10^{19}\mathrm{cm}^{-3}$ is the number den-

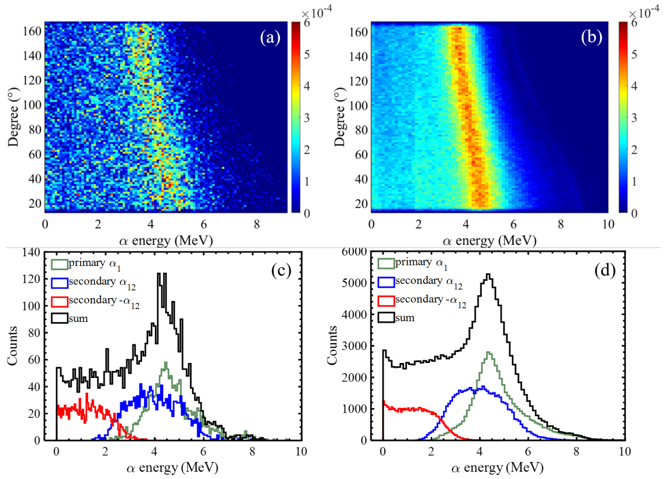


FIG. 7. (a) and (b) Augular distributions of $\alpha-$particle beams in high and low proton intensities from Geant4, respectively. (c) and (d) The energy spectra of $\alpha$ particles in the above conditions along the direction of 52°.

sity of $^{11}$B nuclei, $\frac{dE}{dx}$ the proton stopping power, $\sigma(E)$ the reaction cross section [S3] and $x$ the proton path length in target. In our irradiation conditions, the p$^{11}$B interactions take place inside the target bulk with homogeneous density and temperature. The target ions are assumed to be at rest in the reactions. Considering the incident proton beam with a broad energy spectrum mostly are able to penetrate the whole target [see the black curve in Fig. 2 (a) in the paper], the total path length is $\Delta x \simeq L = 1$ mm with $L$ of the target thickness. Thus the integral fusion probalility can be estimated as $P \simeq n_B L \int_{E_1}^{E_2} \sigma(E) dE = 7.3 \times 10^{-7}$. Then the $\alpha$-particle yield per steradian is about $N_\alpha \simeq 2.2 \times 10^4$/sr in our situation, corresponding to the measured result from the low proton intensity case.

By employing Geant4 computation, the augular distributions of the simulated $\alpha-$particle yields from the foam targets at different proton intensities are present in Fig. 7 (a) and (b). The $\alpha-$particle distributions are anisotropic with high-energy particles or energy peaks mainly occured at the front side of the target. A clear peak around the energy of 4-5 MeV is observed along the direction of 52°. The detected $\alpha-$particle yield with low proton intensity at the 52° direction is about $2.3 \times 10^4$/sr and the yield per proton is $\sim 1.8 \times 10^{-7}$, which is coincident with the measured yield under the same condition [see Table I in the paper]. However, when the incident proton intensity is increased to $\sim 10^{12}$, the corresponding $\alpha-$particle yield is only enhanced by one order of magnitude. This is far less than the measured $\alpha-$particle yield as shown in blue line in Fig. 2 (b) in the paper, which may result from the strong electric fields and induced non-equilibrum thermonuclear reactions between background protons and boron particles. In addition, considering the anisotropic augular distributions of the simulated $\alpha$ particles, the $\alpha$-particle total yields per proton at these two cases in experiment can be estimated as $\sim 3.8 \times 10^{-6}$ and $\sim 6.8 \times 10^{-3}$, which are correponding to the measured results with uniform statistics at $4\pi$ full space.


[S1] Y. W. Liu, X. L. Zhu, Y. L. Gao *et al.*, Quasi suppression of higher-order diffractions with inclined rectangular apertures gratings, Sci. Rep. **5**, 16502 (2015).

[S2] N. M. Shaikh, S. Hafeez, B. Rashid, S. Mahmood, and M. A. Baig, Optical emission studies of the mercury plasma generated by the fundamental, second and third harmonics of a Nd: YAG laser, J. Phys. D **39**, 4377-4385 (2006).

[S3] W. Nevins and R. Swain, The thermonuclear fusion rate coefficient for p-$^{11}$B reactions, Nucl. Fusion **40**, 865 (2000).
